# Supplementary material for: Scheduling and Power Control for V2V Broadcast Communications with Co-Channel and Adjacent Channel Interference
Source: arXiv:1708.02444 ancillary file (2018-12-20)
Supplement: Supplementary file 1 [file Additional_Results.pdf]

# Additional Results of Scheduling and Power Control for V2V BroadcastCommunications with Co-Channel and Adjacent Channel Interference

Anver Hisham, Erik G. Ström, Fredrik Brännström, and Li Yan
Department of Electrical Engineering, Chalmers University of Technology, Gothenburg, Sweden
*{anver, erik.strom, fredrik.brannstrom, lyaa}@chalmers.se*

## I. Introduction

This report presents all the results for the paper [1]. In the paper, due to the page limitations, we presented results only for half-duplex communication and when the adjacent channel interference ratio (ACIR) model is same as the mask specified by 3GPP. Whereas, in this report we present results for both half-duplex and full-duplex communication [1]. Moreover, we present results for the scenarios when the ACIR equals to the mask specified by 3GPP and the single carrier frequency division multiple access (SCFDMA) ACIR model explained in [1].

Using advanced self-interference cancellation techniques, one can achieve self-interference suppression of 113 dB as shown in [2]. We observe that, with this level of self-interference suppression, the adjacent channel self-interference (i.e., self-interference from a transmitting frequency band to adjacent frequency bands) is negligible compared to the inter-VUE signal power. Therefore, for the full-duplex communication scenario, we ignore self-interference by setting the self-channel to zero, i.e., $H_{j,j} = 0 \; \forall j$.

In Section II, Figs. 1–2 present results for half-duplex communication with ACIR equals to the 3GPP mask. In Fig. 1(a), we plot the average number of successful links for various scheduling algorithms, by varying the number of timeslots $T$. Similarly, in Fig. 1(b) and Fig. 1(c), we plot the same by varying the number of frequency slots $F$ and number of vehicular user equipments (VUEs) $N$, respectively. In Figs. 1(a)–(c), we used equal power for all VUEs. Similarly, we plot the results for our heuristic power control and near-optimal power control in Figs. 1(d)–(f) and Figs. 1(g)–(i) respectively.

Fig. 2 presents the average transmit power of a VUE for various scheduling and power control algorithms. Figs. 2(a)–(c) show the transmit power for the BIS with $w = 1$. Similarly, we show the results for BIS (optmized $w$), heuristic scheduling, and near-optimal scheduling in Figs. 2(d)–(f), Figs. 2(g)–(i), and Figs. 2(j)–(l), respectively.

In Section III, we present the results for half-duplex communication when the ACIR model equals to the SCFDMA ACIR model, which is shown in [1, Fig. 3]. Similarly, in Sections IV and V, we present results for full-duplex communication when the ACIR equals to the ACIR mask in 3GPP and SCFDMA ACIR model, respectively.

We have not simulated near-optimal scheduling for $T > 1$, due to its very high computational complexity. Therefore, the corresponding results are not included. Moreover, in the half-duplex scenario we schedule only upto half of the VUEs when $T = 1$. However, for the full-duplex scenario, we consider all VUEs for scheduling when $T = 1$.

## References

[1] Anver Hisham, Erik G. Ström, Fredrik Brännström, and Li Yan "Scheduling and power control for broadcast V2V communications with co-channel and adjacent channel interference" Aug. 2017, [Online]. Available: https://arxiv.org/abs/1708.02444
[2] L. Wang, F. Tian, T. Svensson, D. Feng, M. Song and S. Li, "Exploiting full duplex for device-to-device communications in heterogeneous networks," in *IEEE Communications Magazine*, vol. 53, no. 5, pp. 146-152, May 2015.

The research was, in part, funded by the Swedish Governmental Agency for Innovation Systems (VINNOVA), FFI - Strategic Vehicle Research and Innovation, under Grant No. 2014-01387. This work has, in part, been performed in the framework of the H2020 project 5GCAR co-funded by the EU. The authors would like to acknowledge the contributions of their colleagues. The views expressed are those of the authors and do not necessarily represent the project. The consortium is not liable for any use that may be made of any of the information contained therein.

## II. HALF-DUPLEX RESULTS WITH 3GPP ACIR MASK

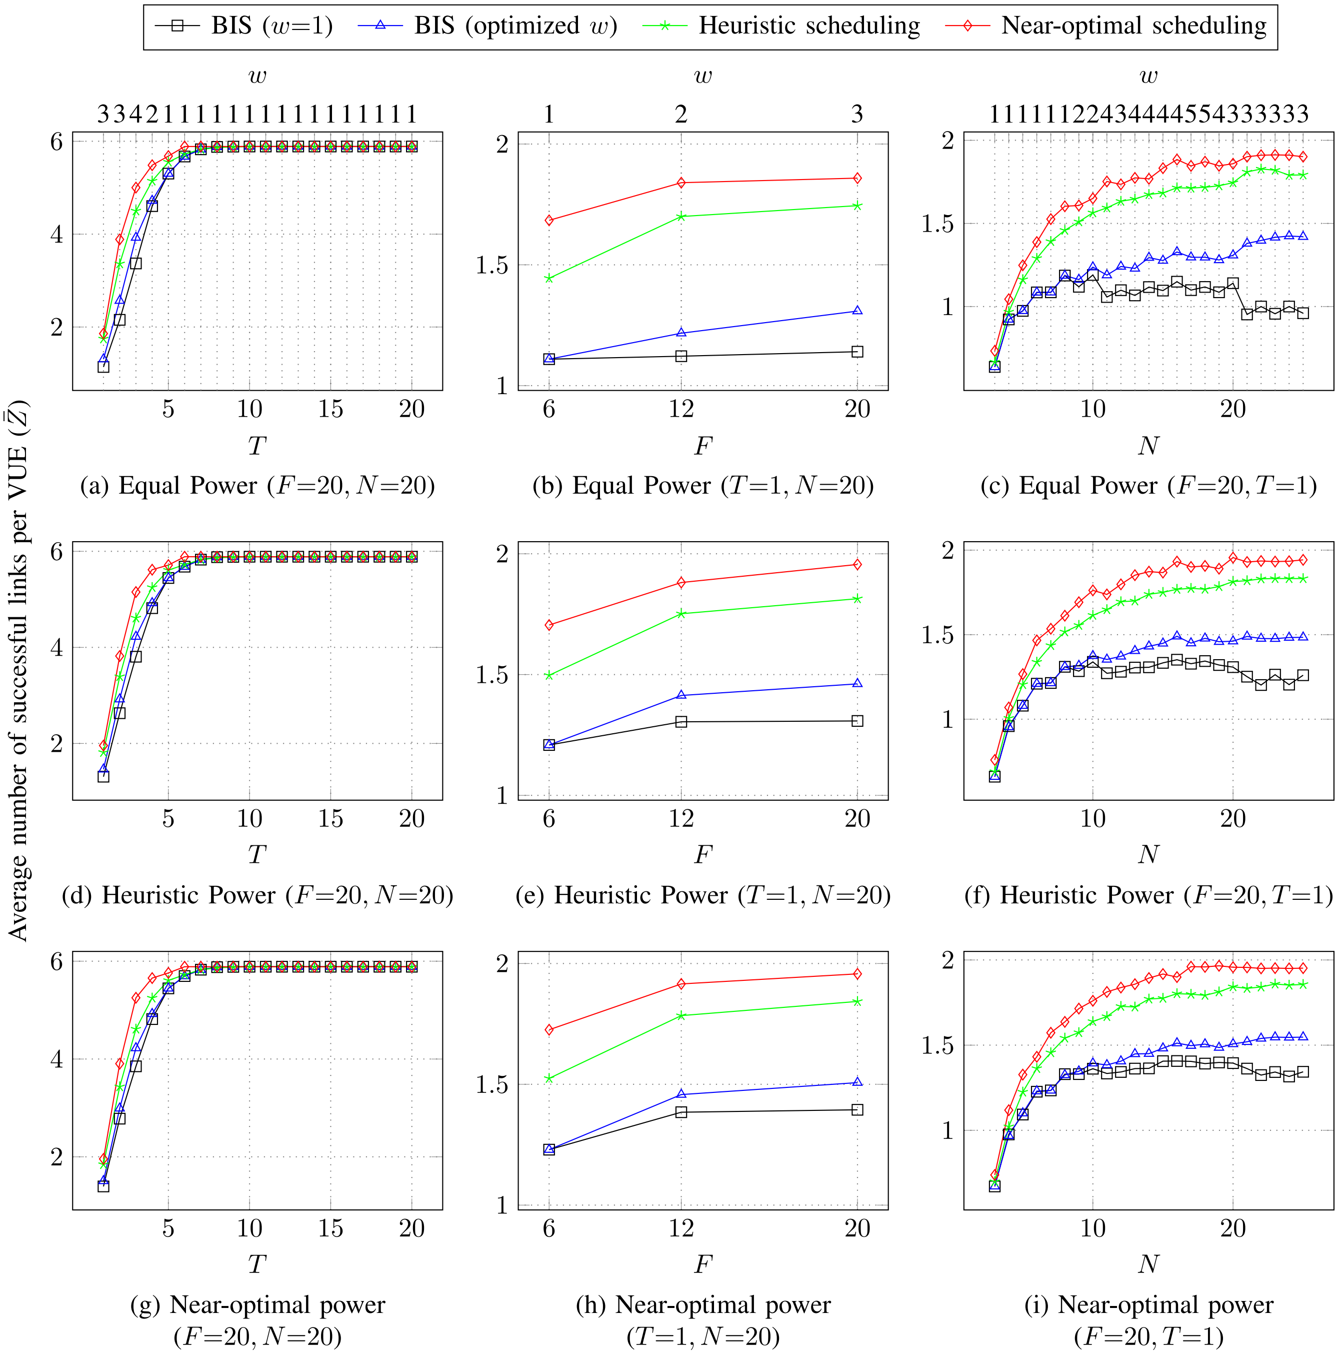


Fig. 1: Average number of successful links per VUE ($\bar{Z}$) for various scheduling algorithms

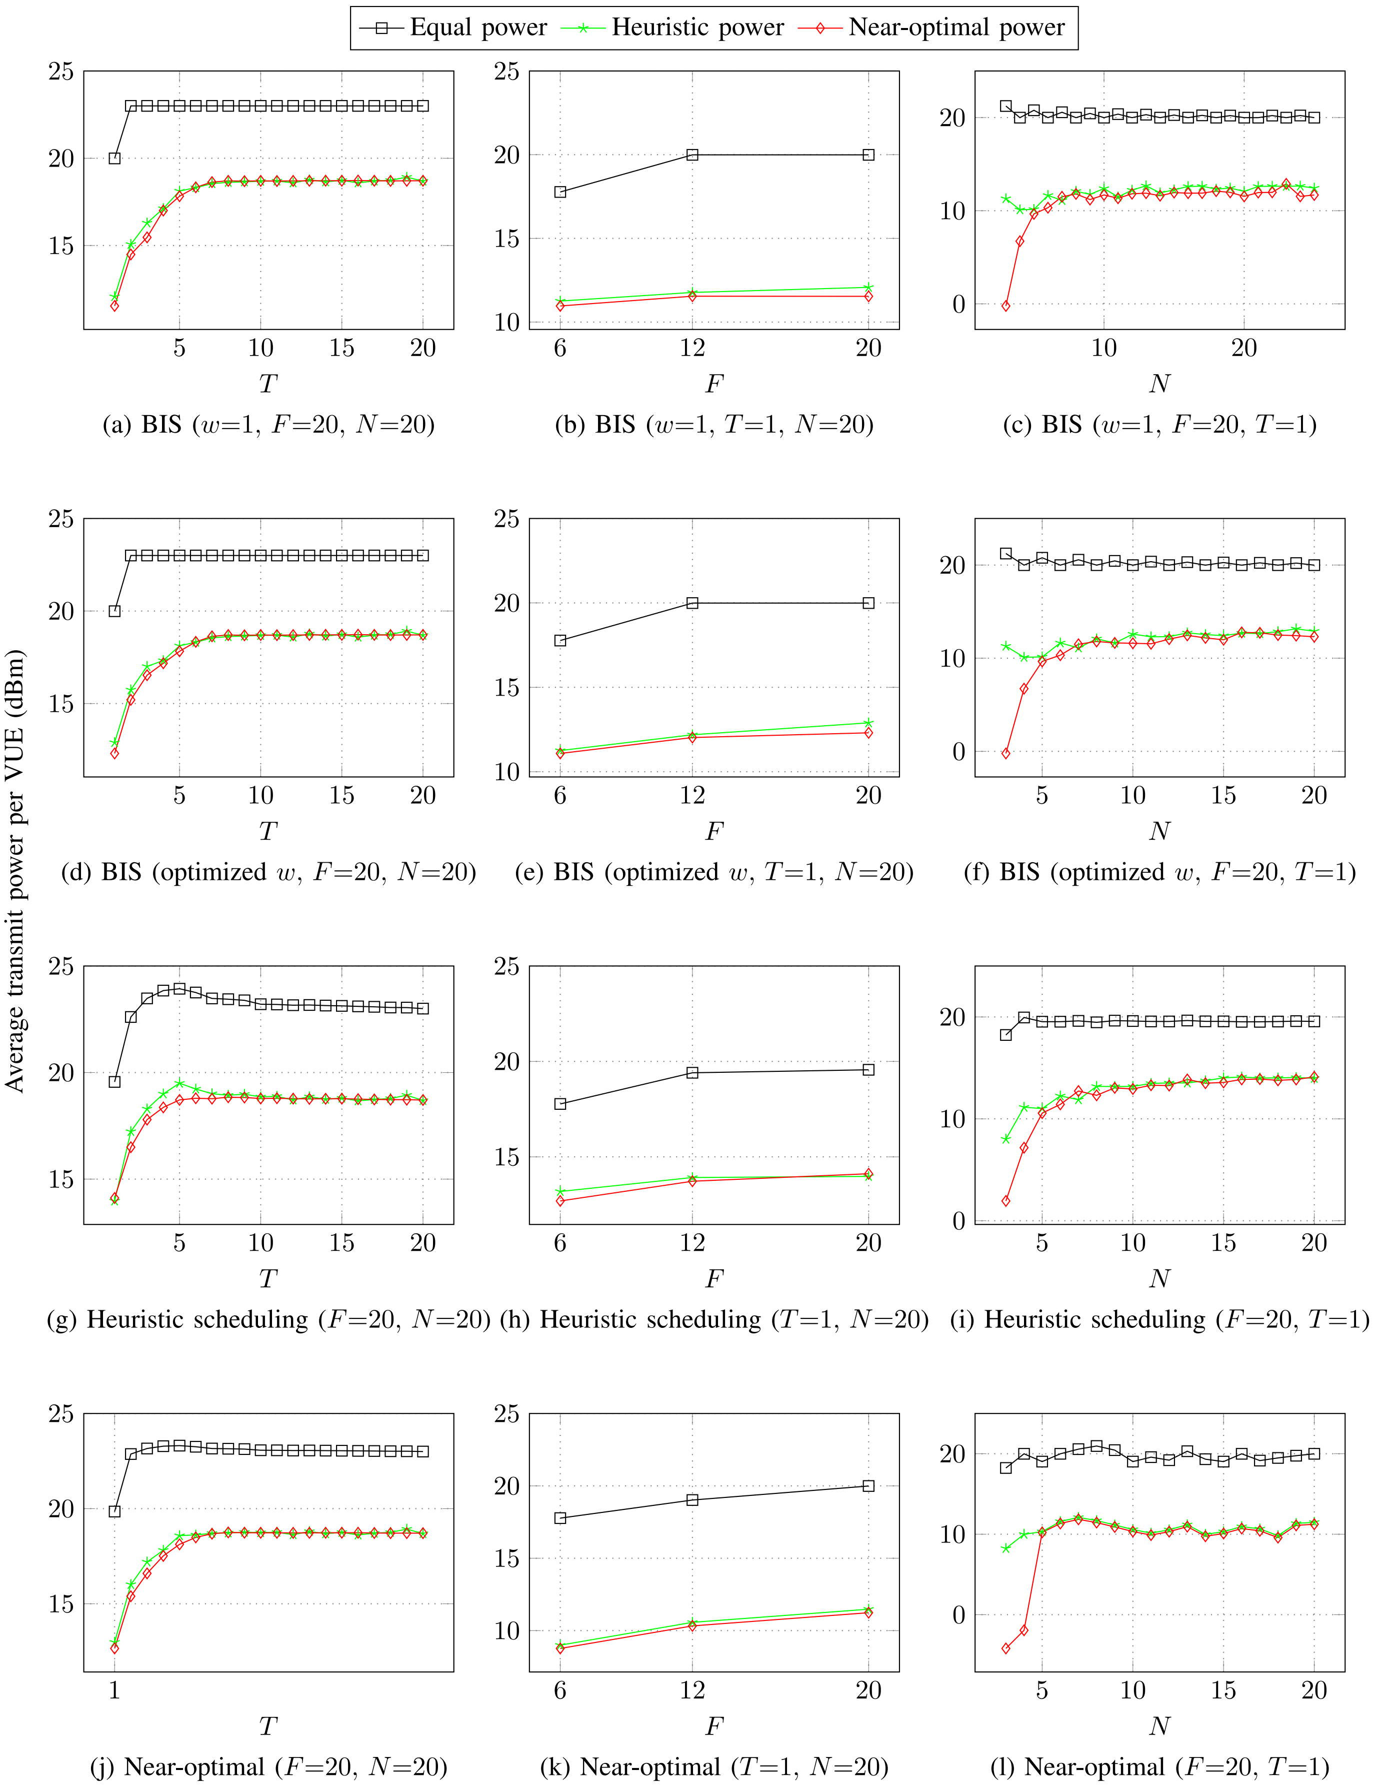


Fig. 2: Average transmit Power for various power control algorithms

## III. Half-Duplex results with SCFDMA ACIR model

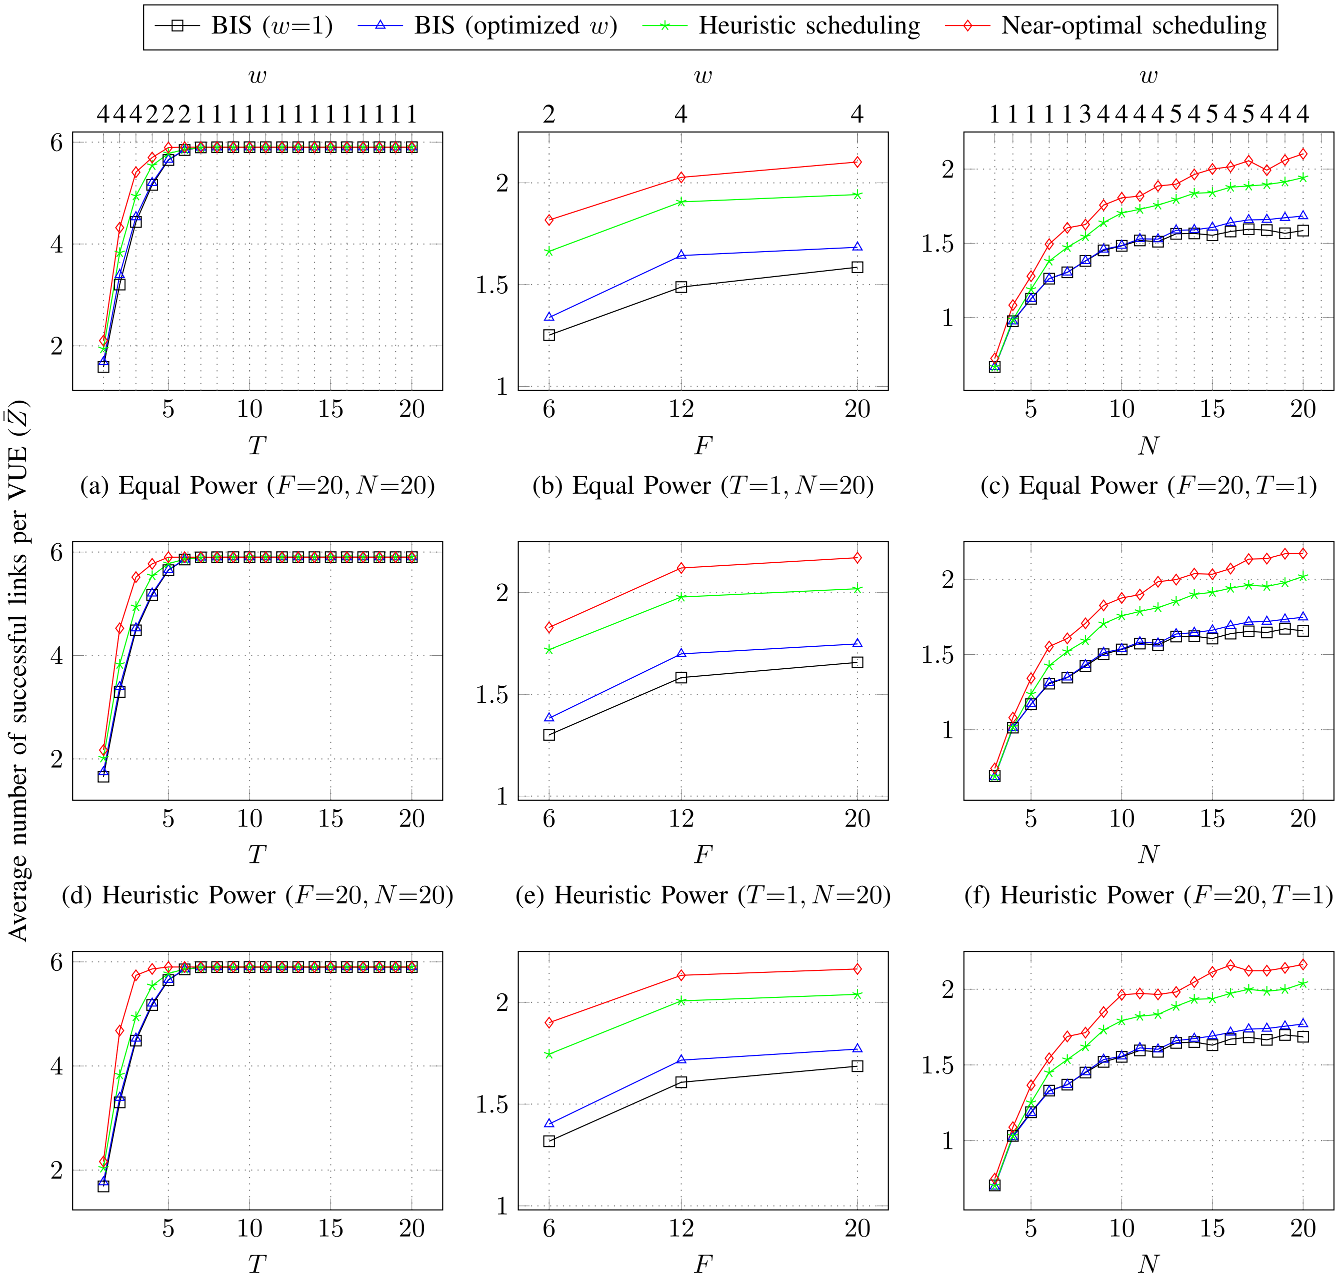


(a) Equal Power ($F$=20, $N$=20)

(b) Equal Power ($T$=1, $N$=20)

(c) Equal Power ($F$=20, $T$=1)

(d) Heuristic Power ($F$=20, $N$=20)

(e) Heuristic Power ($T$=1, $N$=20)

(f) Heuristic Power ($F$=20, $T$=1)

(g) Near-optimal power ($F$=20, $N$=20)

(h) Near-optimal power ($T$=1, $N$=20)

(i) Near-optimal power ($F$=20, $T$=1)

Fig. 3: Average number of successful links per VUE ($\bar{Z}$) for various scheduling algorithms

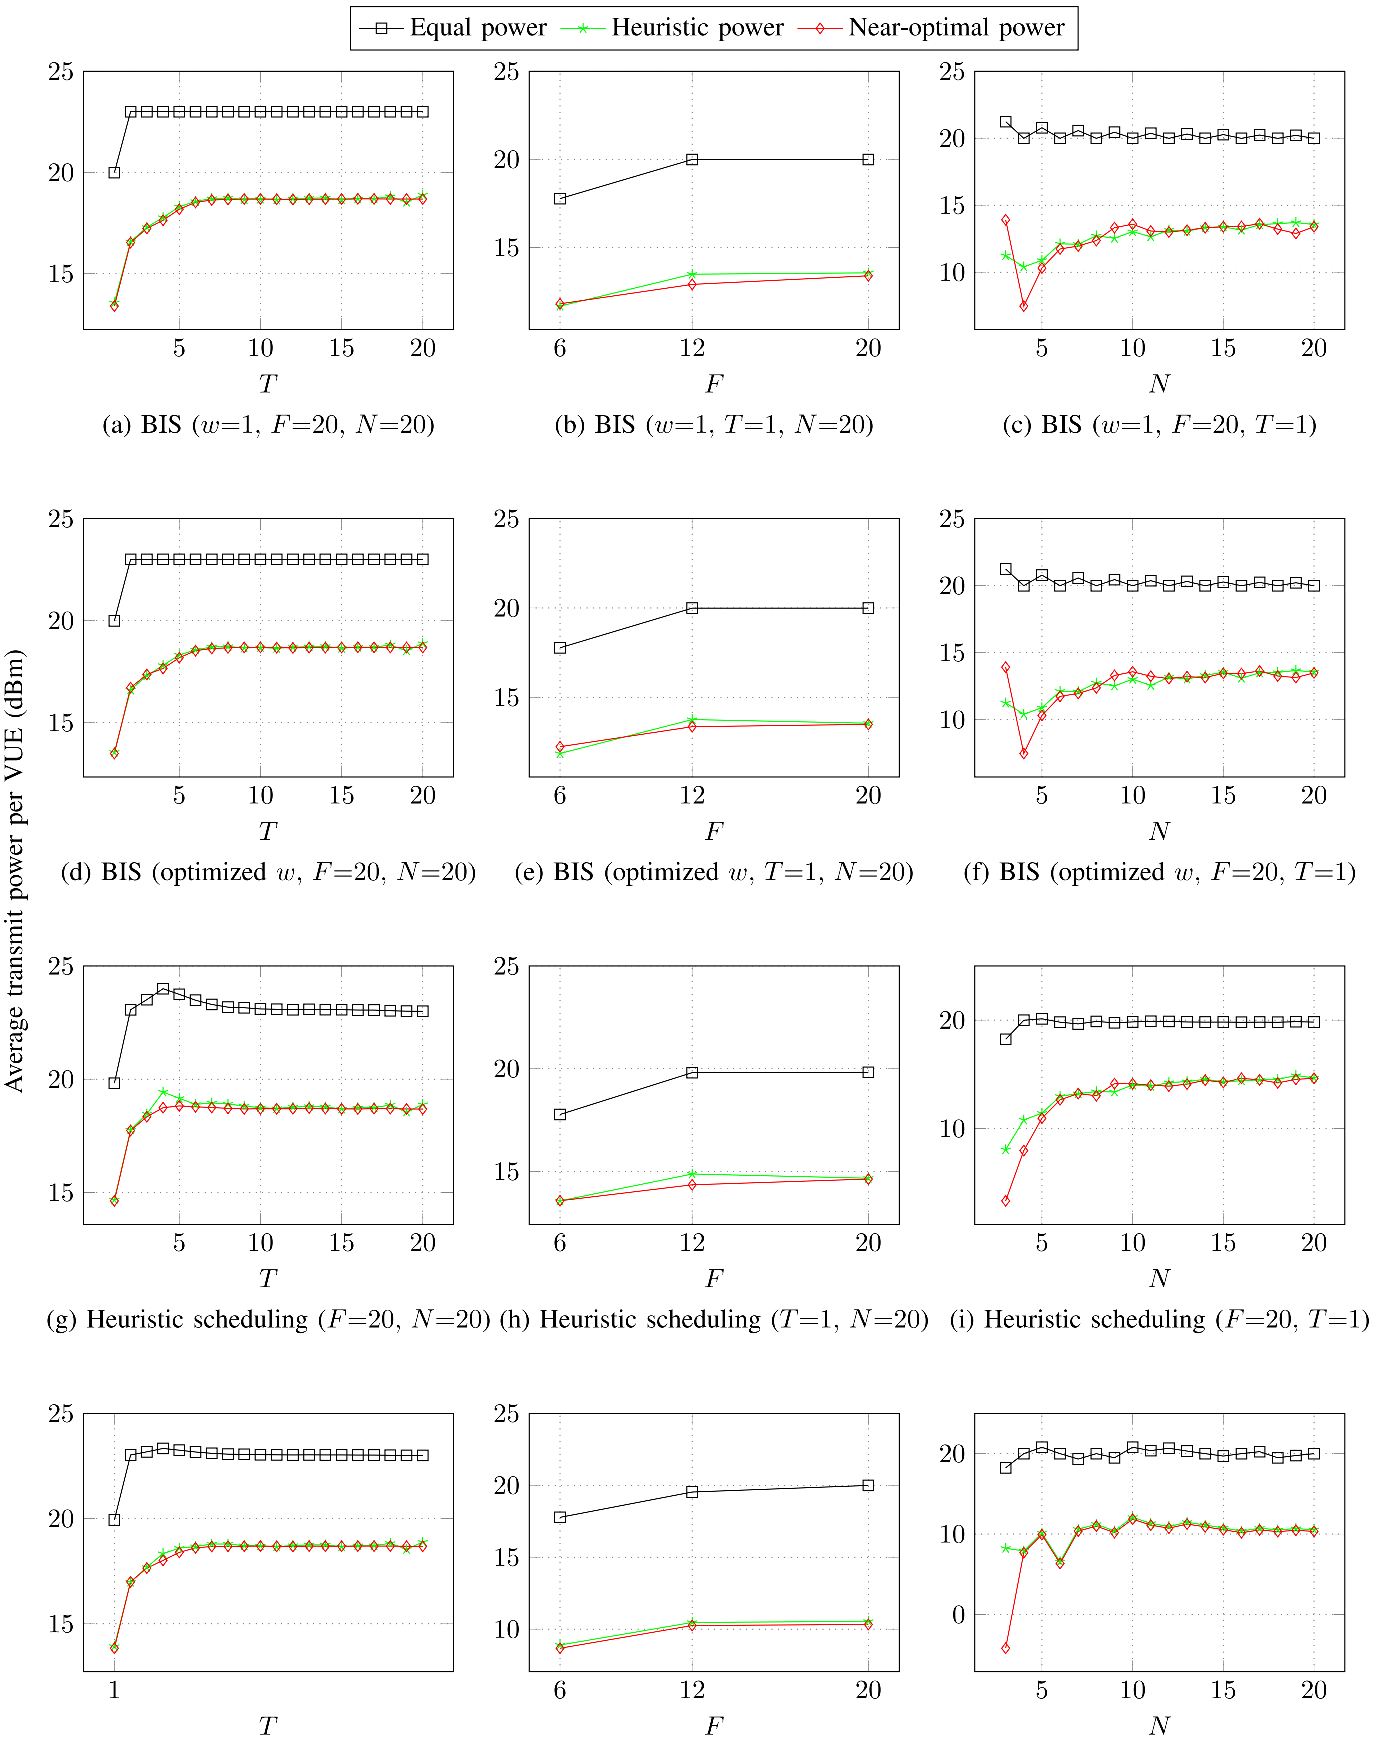


(a) BIS ($w$=1, $F$=20, $N$=20) (b) BIS ($w$=1, $T$=1, $N$=20) (c) BIS ($w$=1, $F$=20, $T$=1)

(d) BIS (optimized $w$, $F$=20, $N$=20) (e) BIS (optimized $w$, $T$=1, $N$=20) (f) BIS (optimized $w$, $F$=20, $T$=1)

(g) Heuristic scheduling ($F$=20, $N$=20) (h) Heuristic scheduling ($T$=1, $N$=20) (i) Heuristic scheduling ($F$=20, $T$=1)

(j) Near-optimal ($F$=20, $N$=20) (k) Near-optimal ($T$=1, $N$=20) (l) Near-optimal ($F$=20, $T$=1)

Fig. 4: Average transmit Power for various power control algorithms

## IV. Full-Duplex results with 3GPP ACIR mask

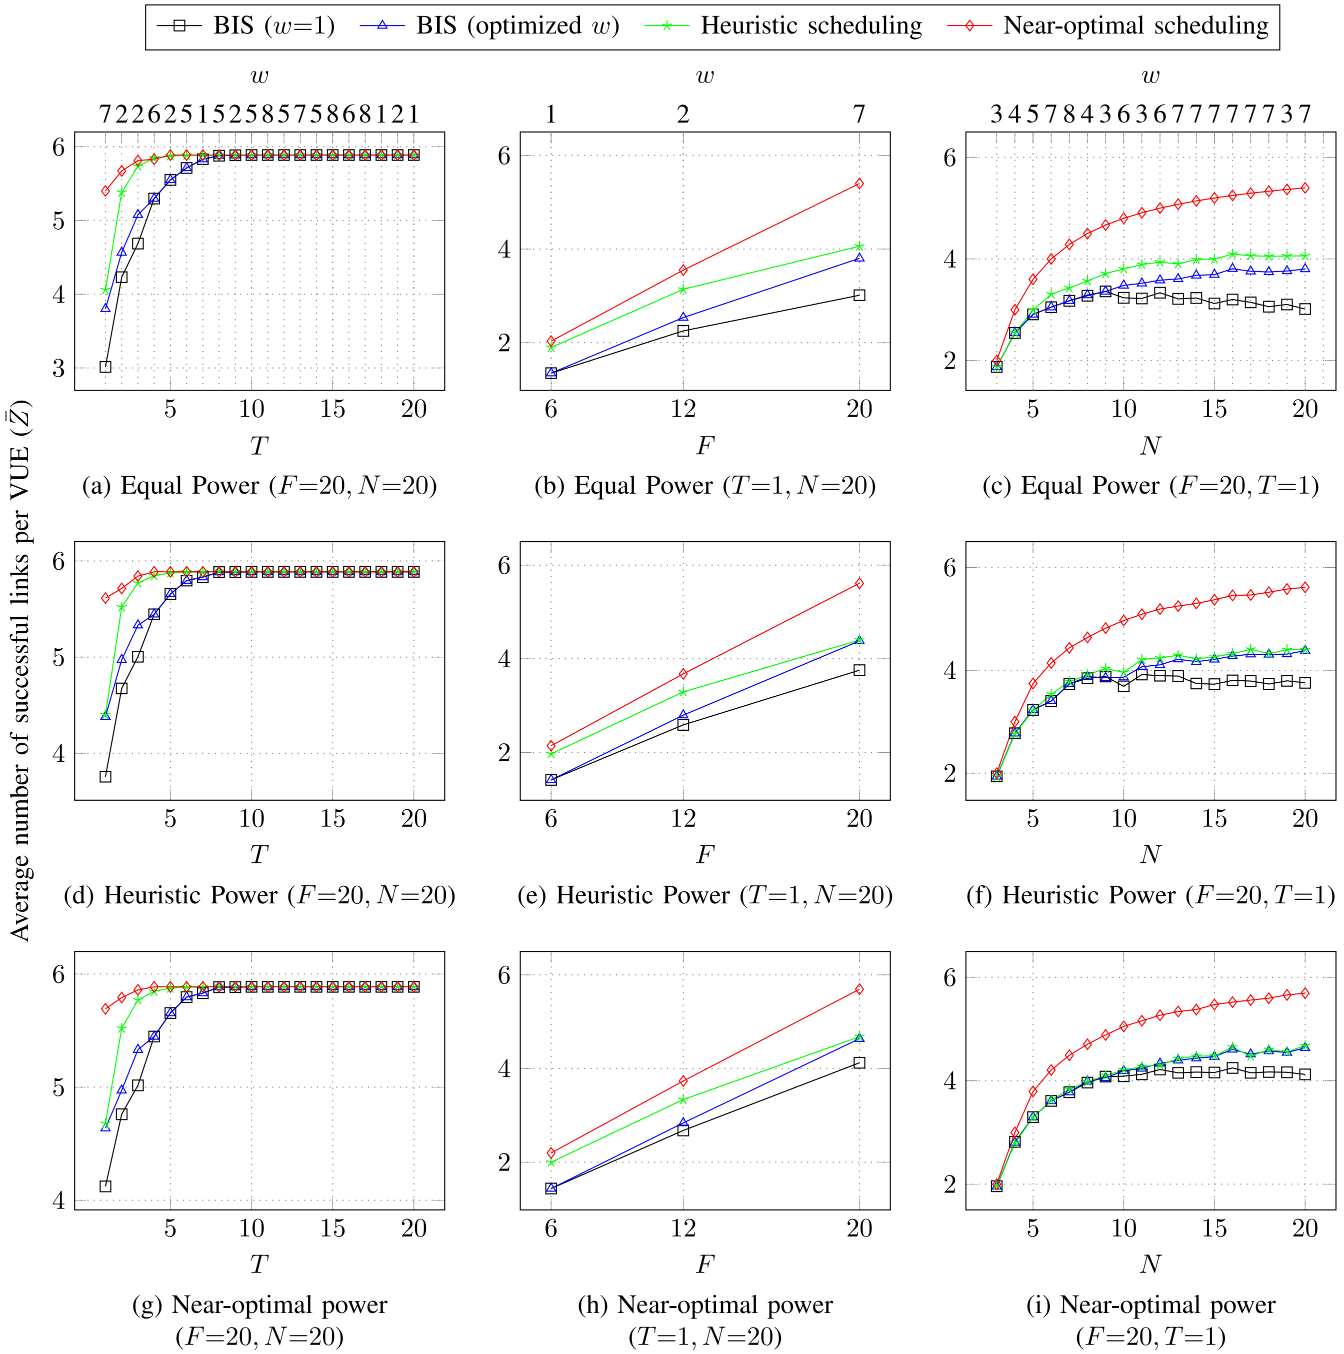


(a) Equal Power ($F$=20, $N$=20)

(b) Equal Power ($T$=1, $N$=20)

(c) Equal Power ($F$=20, $T$=1)

(d) Heuristic Power ($F$=20, $N$=20)

(e) Heuristic Power ($T$=1, $N$=20)

(f) Heuristic Power ($F$=20, $T$=1)

(g) Near-optimal power ($F$=20, $N$=20)

(h) Near-optimal power ($T$=1, $N$=20)

(i) Near-optimal power ($F$=20, $T$=1)

Fig. 5: Average number of successful links per VUE ($\bar{Z}$) for various scheduling algorithms

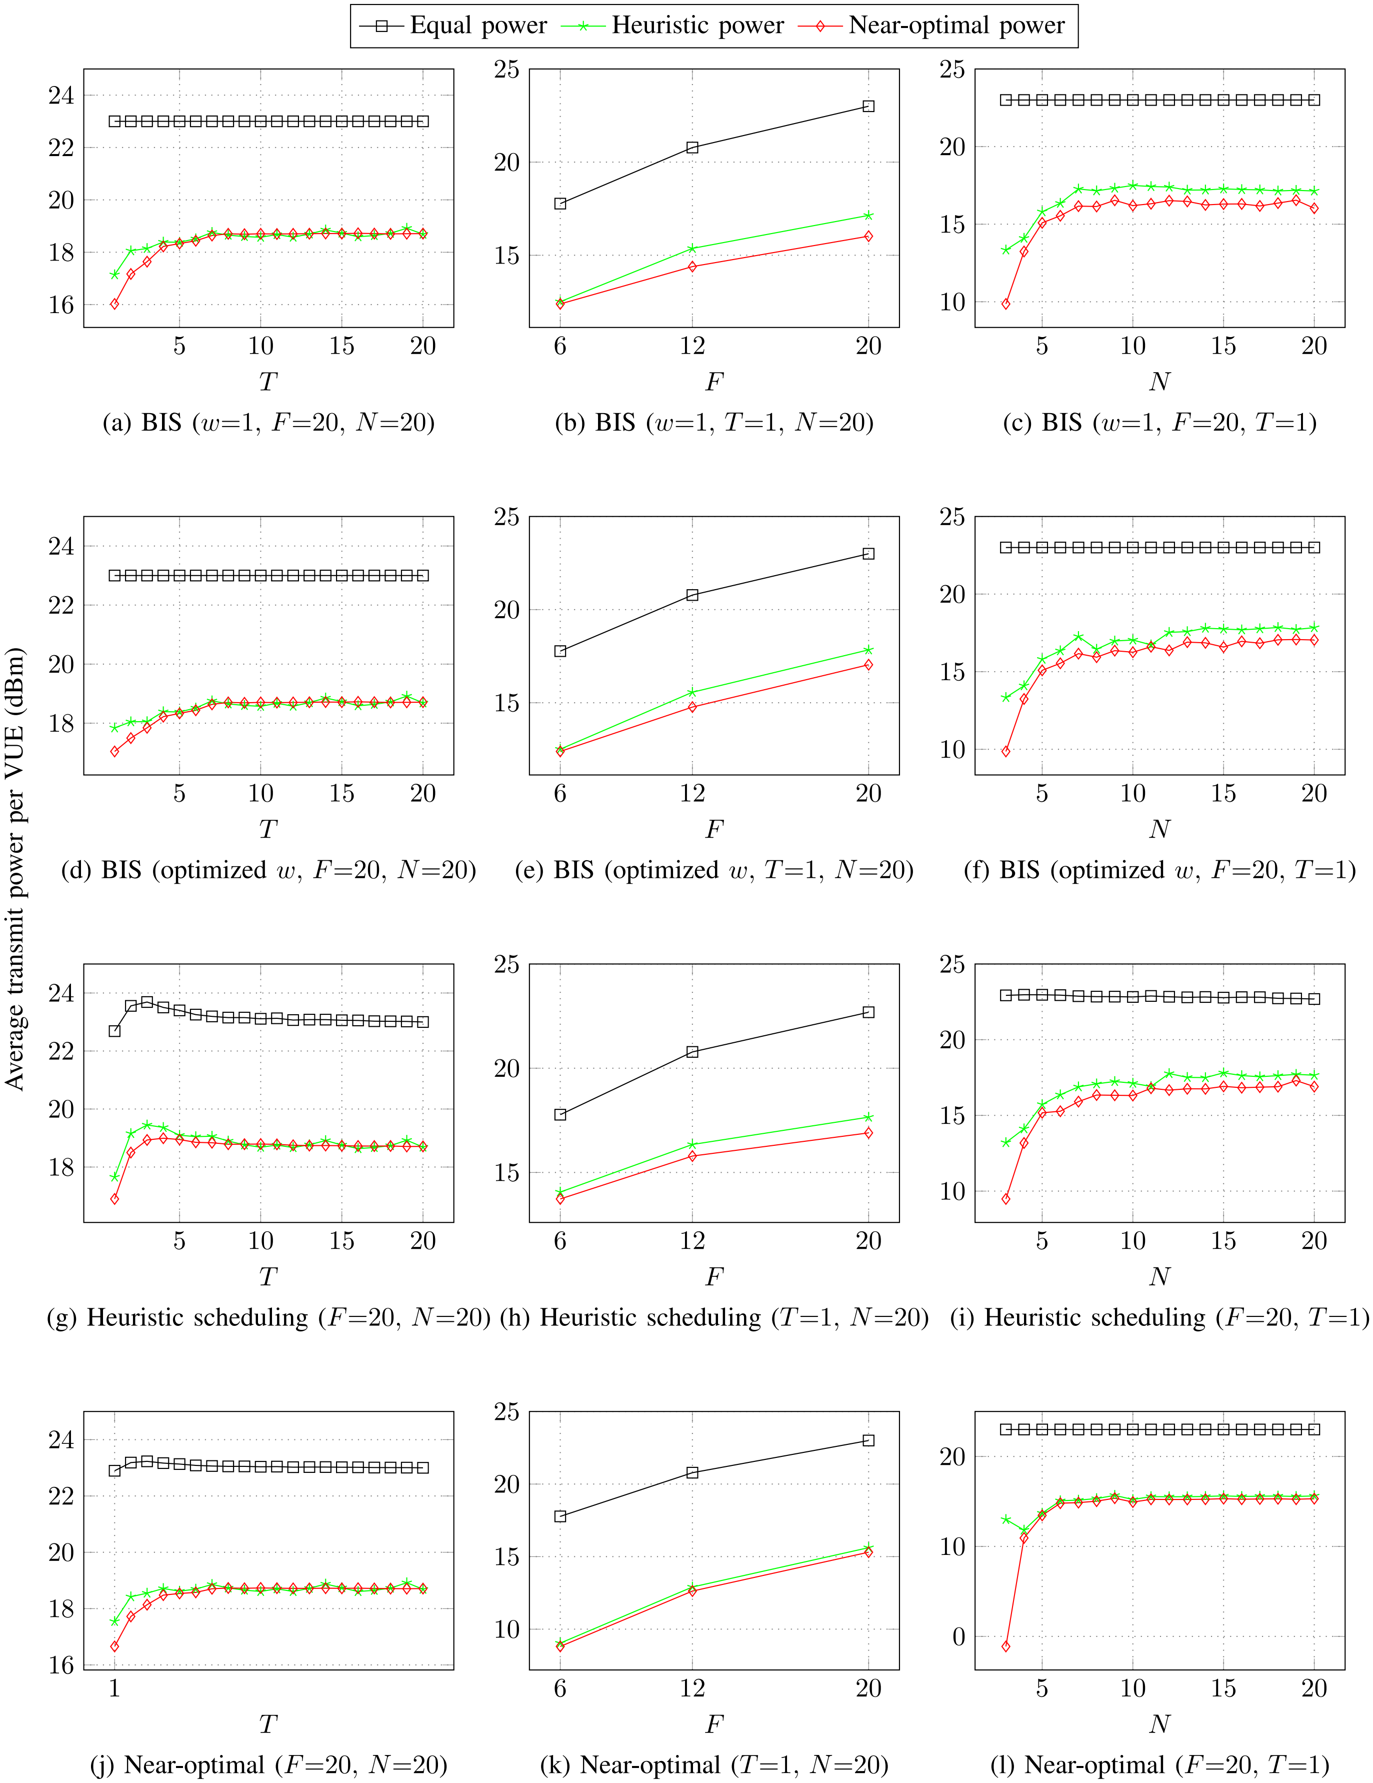


(a) BIS ($w$=1, $F$=20, $N$=20) (b) BIS ($w$=1, $T$=1, $N$=20) (c) BIS ($w$=1, $F$=20, $T$=1)

(d) BIS (optimized $w$, $F$=20, $N$=20) (e) BIS (optimized $w$, $T$=1, $N$=20) (f) BIS (optimized $w$, $F$=20, $T$=1)

(g) Heuristic scheduling ($F$=20, $N$=20) (h) Heuristic scheduling ($T$=1, $N$=20) (i) Heuristic scheduling ($F$=20, $T$=1)

(j) Near-optimal ($F$=20, $N$=20) (k) Near-optimal ($T$=1, $N$=20) (l) Near-optimal ($F$=20, $T$=1)

Fig. 6: Average transmit Power for various power control algorithms

## V. Full-Duplex results with SCFDMA ACIR model

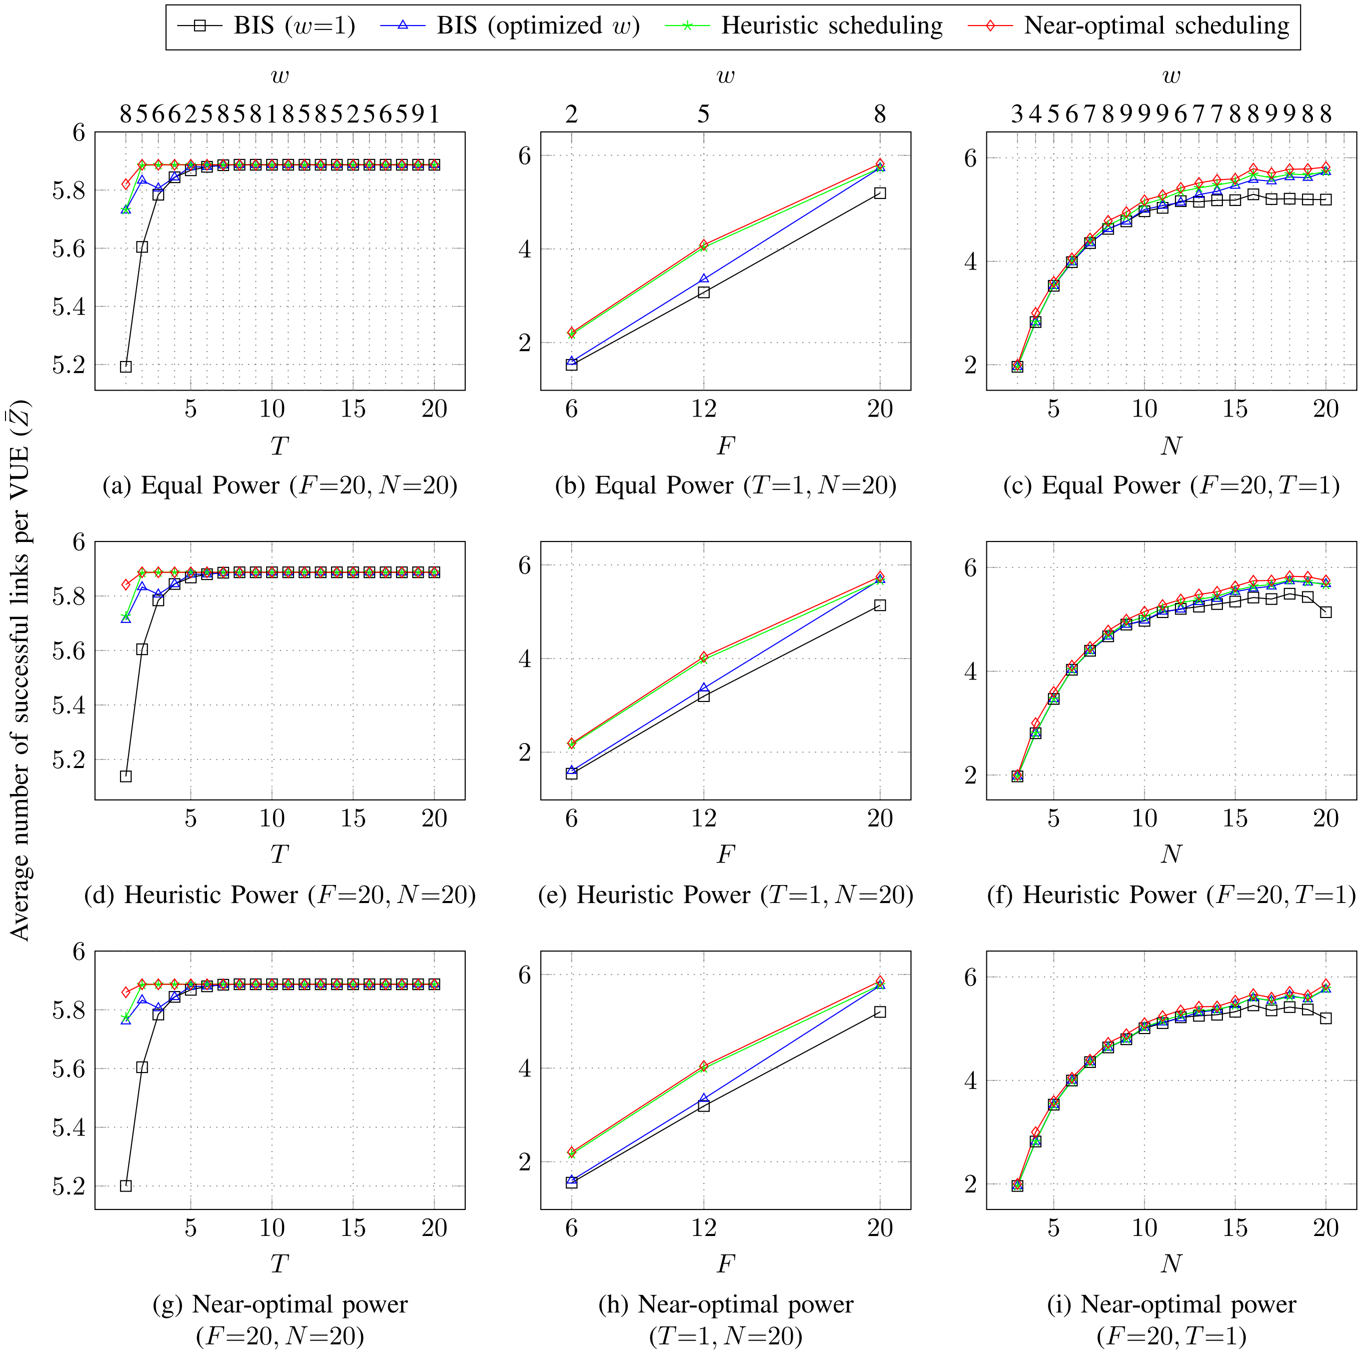


(a) Equal Power ($F$=20, $N$=20)
(b) Equal Power ($T$=1, $N$=20)
(c) Equal Power ($F$=20, $T$=1)
(d) Heuristic Power ($F$=20, $N$=20)
(e) Heuristic Power ($T$=1, $N$=20)
(f) Heuristic Power ($F$=20, $T$=1)
(g) Near-optimal power ($F$=20, $N$=20)
(h) Near-optimal power ($T$=1, $N$=20)
(i) Near-optimal power ($F$=20, $T$=1)

Fig. 7: Average number of successful links per VUE ($\bar{Z}$) for various scheduling algorithms

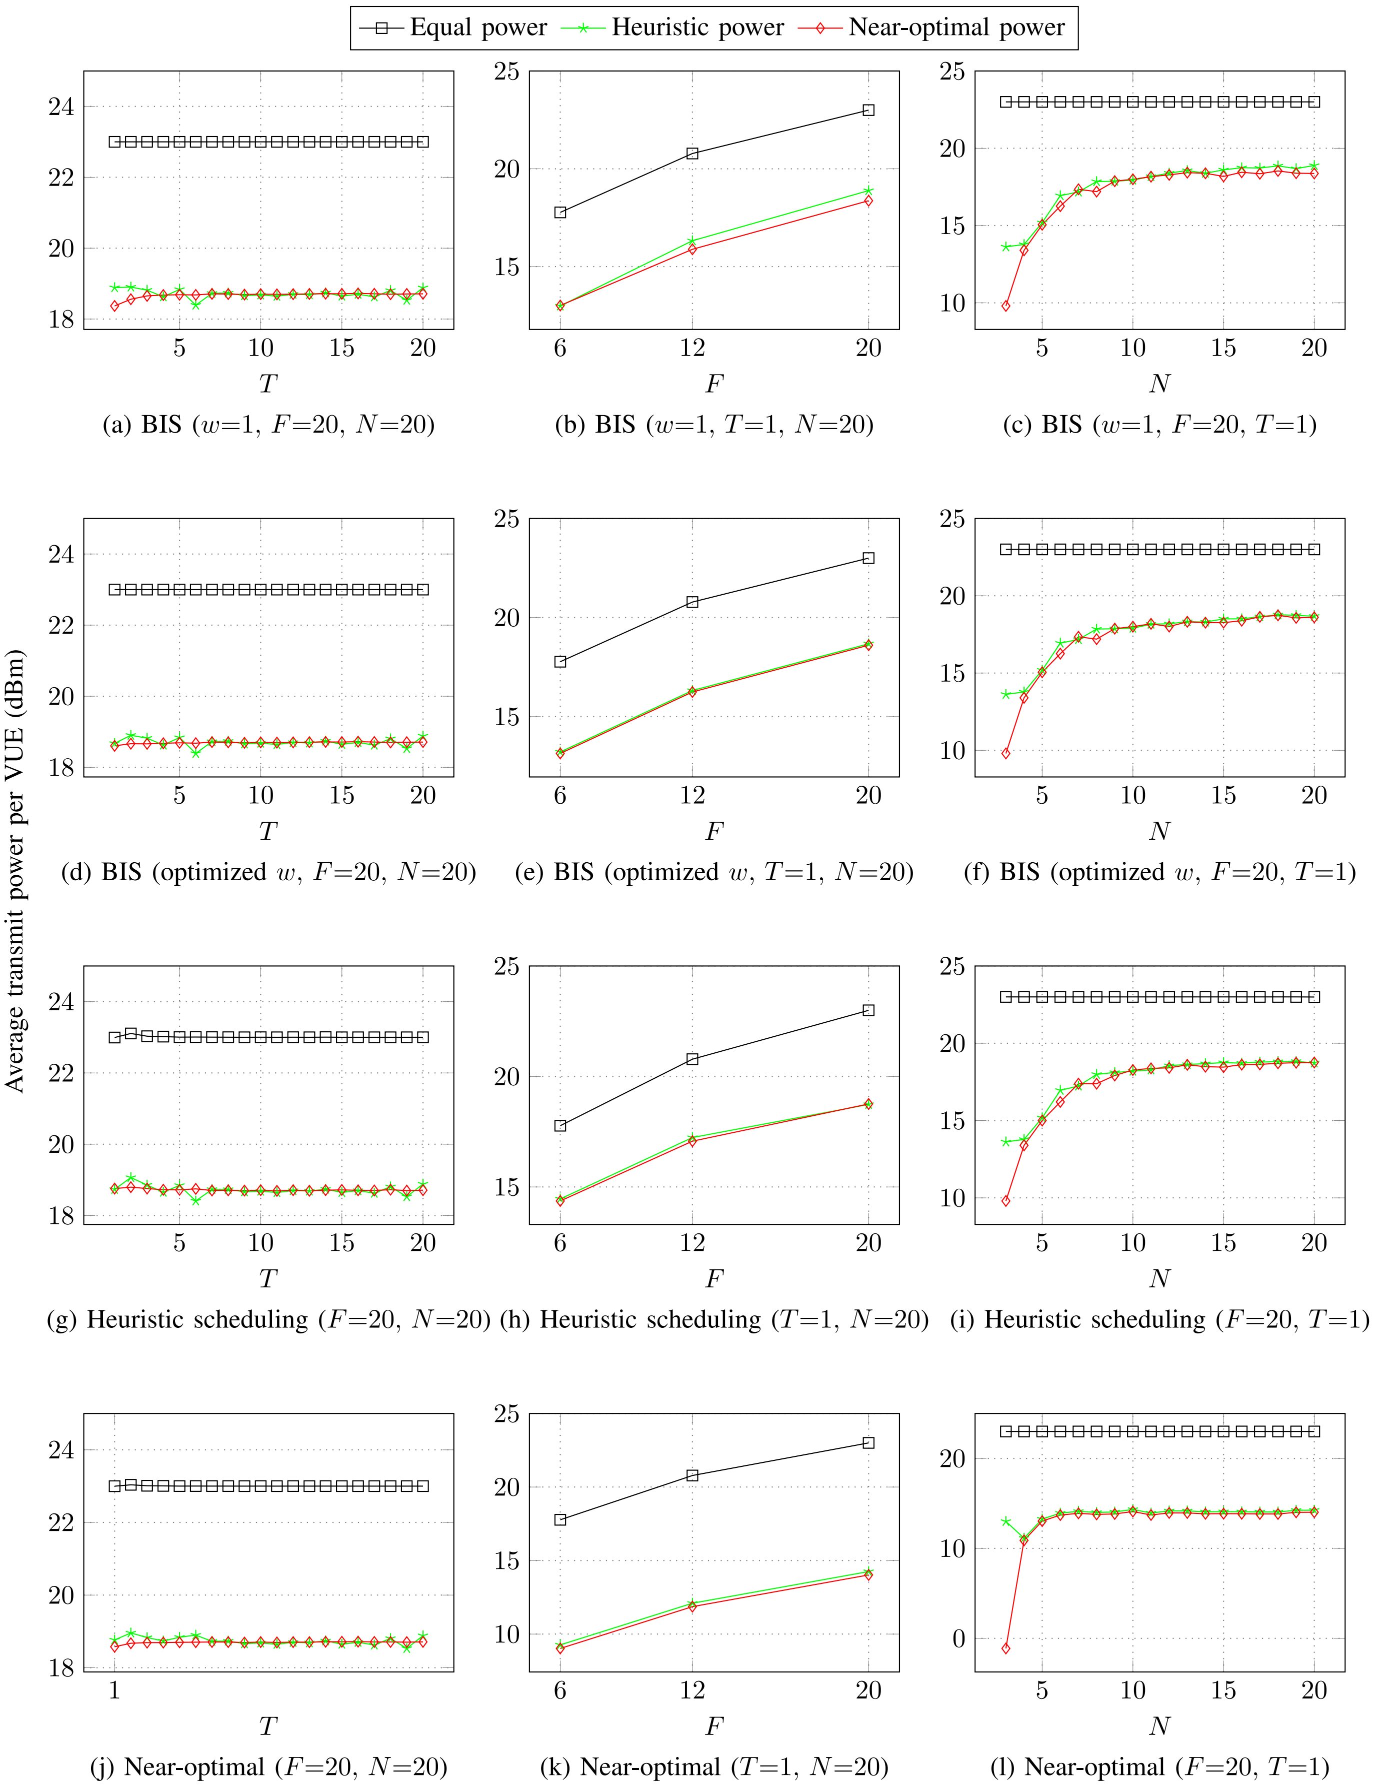


Fig. 8: Average transmit Power for various power control algorithms
